# Supplementary material for: Characterizing and Extending Answer Set Semantics using Possibility Theory
Source: arXiv:1312.0127 source file (2013-11-30)
Supplement: Supplementary file 1 [file appendix.pdf]

Online appendix for the paper

# *Characterizing and Extending Answer Set Semantics using Possibility Theory*

published in Theory and Practice of Logic Programming

KIM BAUTERS
*Department of Applied Mathematics, Computer Science and Statistics, Universiteit Gent*
*Krijgslaan 281 (WE02), 9000 Gent, Belgium*
(*e-mail:* kim.bauters@gmail.com)

STEVEN SCHOCKAERT
*School of Computer Science & Informatics, Cardiff University*
*5 The Parade, Cardiff CF24 3AA, United Kingdom*
(*e-mail:* s.schockaert@cs.cardiff.ac.uk)

MARTINE DE COCK
*Department of Applied Mathematics, Computer Science and Statistics, Universiteit Gent*
*Krijgslaan 281 (WE02), 9000 Gent, Belgium*
(*e-mail:* martine.decock@ugent.be)

DIRK VERMEIR
*Department of Computer Science, Vrije Universiteit Brussel,*
*Pleinlaan 2, 1050 Brussel, Belgium*
(*e-mail:* dirk.vermeir@vub.ac.be)

*submitted 20 March 2012; revised 19 August 2013; accepted 5 November 2013*

## Proofs

*Lemma 1*

constraintsEquivalent Let $L$ be a set of literals, $M \subseteq L$ a consistent set of literals and let the possibility distribution $\pi$ be defined as $\pi(\omega) = 1$ if $\omega \models M$ and $\pi(\omega) = 0$ otherwise. Then $M = \{l \mid N(l) = 1, l \in L\}$.

*Proof*

It is easy to see that for every $l \in M$ we have $N(l) = 1$. Indeed, assume that $l \in M$. Then $\omega \models \neg l$ (which is equivalent to $\omega \not\models l$) implies $\omega \not\models M$, and, by the definition of $\pi$, that $\pi(\omega) = 0$. We thus obtain

$$N(l) = 1 - \Pi(\neg l) = 1 - \max\{\pi(\omega) \mid \omega \models \neg l\} = 1.$$

Furthermore, for every $l \notin M$ we must have $N(l) = 0$. Indeed, assume that $l \notin M$, then $M \cup \{\neg l\}$ is consistent. Thus there exists a world $\omega_0$ such that $\omega_0 \models (M \cup \{\neg l\})$, i.e. $\omega_0 \models M$ and $\omega_0 \models \neg l$, or, by the definition of $\pi$, $\pi(\omega_0) = 1$ and $\omega_0 \models \neg l$. We thus

obtain

$$N(l) = 1 - \Pi(\neg l) = 1 - \max\{\pi(\omega) \mid \omega \models \neg l\}$$
$$\leq 1 - \pi(\omega_0) = 0$$

Since, by construction of $\pi$, $N(l)$ is either 0 or 1, this concludes the proof. □

*Proposition 1*
Let $P$ be a simple program. If $\pi \in S_P$ then either the unique consistent answer set of $P$ is given by $M = \{l \mid N(l) = 1, l \in Lit_P\}$ or $\pi$ is the vacuous distribution, in which case $P$ does not have any consistent answer sets.

*Proof*
We can write the simple program $P$ as $P = P' \cup C$ with $C$ the set of constraint rules and $P'$ the set of all the remaining rules. Since $\pi \in S_P$, we also know that for every rule $r \in P$ we have that $\pi$ satisfies the constraint $\gamma(r)$.
We now consider the two cases stated in the proposition:

- $\exists \omega \in \Omega \cdot \pi(\omega) > 0$ (i.e. $\pi$ is not the vacuous distribution)
  This implies that there is no constraint rule $r \in C$ that is violated by the answer set $M$. Indeed, we cannot have for a constraint rule $r = (\leftarrow l_1, ..., l_m)$ that $N(l_1) = ... = N(l_m) = 1$ since $\gamma(r)$ would then imply that $N(\bot) = 1$, i.e. $\forall \omega \in \Omega \cdot \pi(\omega) = 0$. Hence we find that $\{l_1, ..., l_m\} \not\subseteq M$ due to the construction of $M$, i.e. $r$ is not violated by $M$. As such, we know for the remainder of this part of the proof that we only need to take the rules in $P'$ into account, as the rules in $C$ are not applicable.
  We now verify that $M$ is a model of $P$. To see this, first recall that every rule $r \in P$ imposes the constraint $\gamma(r) = N(l_0) \geq \min(N(l_1), ..., N(l_m))$. Thus, whenever $N(l_1) = ... = N(l_m) = 1$ we know that $\gamma(r)$ enforces that $N(l_0) = 1$. Since $\pi$ satisfies $\gamma(r)$ and due to the construction of $M$ we thus have that $l_0 \in M$ whenever $\{l_1, ..., l_m\} \subseteq M$, i.e. $M$ is a model of $P$.
  In addition, we can show that $M$ is a consistent model. If $M$ were not a consistent model, then there would be a literal $l$ such that both $l \in M$ and $\neg l \in M$. Thus, by construction of $M$, we would have that $N(l) = 1$ and $N(\neg l) = 1$. In this case we have $\min(N(l), N(\neg l)) = 1$ and, because of the min-decomposability of $N$ w.r.t. conjunction, $N(l \wedge \neg l) = 1$. This would imply that $N(\bot) = 1$ i.e. we would have that $\forall \omega \in \Omega \cdot \pi(\omega) = 0$. Since we assumed that this is not the case, we must have that $M$ is a consistent model.
  We can now verify that $M$ is a minimal model. To see this, assume that $M$ is a consistent model, but not a minimal model of $P$. Since $M$ is not a minimal model, we know that there exists another consistent model $M'$ of $P$ such that $M' \subset M$. Let us take $\pi'$ such that $\pi'(\omega) = 1$ if $\omega \models M'$ and $\pi'(\omega) = 0$ otherwise. From Lemma 1 we obtain that $M' = \{l \mid N'(l) = 1, l \in Lit_P\}$ with $N'$ the necessity measure induced by $\pi'$. We then have that $\pi' \in C_P$. Indeed, by assumption $M'$ is a model and thus for every rule $r \in P$ with $r = (l_0 \leftarrow l_1, ..., l_m)$ we have $l_0 \in M'$ whenever $\{l_1, ..., l_m\} \subseteq M'$. Due to

the relationship between $M'$ and $N'$ and since for every literal $l$ we know that $N'(l) \in \{0, 1\}$ by construction, we have that $\pi'$ satisfies the constraint $\gamma'(r) = N'(l_0) \geq \min(N'(l_1), ..., N'(l_m))$ imposed by every rule $r \in P$ and hence $\pi' \in C_P$.
We now show that $M' \subset M$ leads to a contradiction. Since $M' \subset M$ we know that there is some literal $l \in M \setminus M'$ with $N'(l) < N(l)$ due to the definitions of $M$ and $M'$. Thus $\exists \omega \in \Omega \cdot \pi'(\omega) > \pi(\omega)$. Furthermore we have that $\forall \omega \in \Omega \cdot \pi'(\omega) \geq \pi(\omega)$ by construction, unless it were the case that $\pi'(\omega) = 0$ while $\pi(\omega) > 0$ for some $\omega$. Given the construction of $M$, we know that whenever $\omega \not\models M$, i.e. whenever for some $l \in M$ we have $\omega \not\models l$ (or equivalently $\omega \models \neg l$), that $\pi(\omega) = 0$ since $l \in M$ implies that $\max\{\pi(\omega) \mid \omega \models \neg l\} = 0$. Hence whenever $\pi(\omega) > 0$, we know that $\omega \models M$. Thus we find $\omega \not\models M'$ by construction and $\omega \models M$, which cannot be the case since $M' \subset M$. Hence we conclude that we must have $\exists \omega \in \Omega \cdot \pi'(\omega) > \pi(\omega)$ and $\forall \omega \in \Omega \cdot \pi'(\omega) \geq \pi(\omega)$, i.e. we find that $\pi \notin S_P$. This is a contradiction; $M$ must therefore be a minimal model of $P$.

- $\forall \omega \in \Omega \cdot \pi(\omega) = 0$
We consider the two possible cases in which a program $P = P' \cup C$ has the vacuous distribution as a minimally specific possibilistic model. In that case, we may have $\pi \in S_{P'}$, i.e. even without considering the constraints, the vacuous distribution is a minimally specific model of the rules in $P'$. Otherwise we have $\pi \in C_P \setminus C_{P'}$, i.e. we need to consider the constraint rules in $C$ to obtain the vacuous distribution.
Assume that $\pi \in S_{P'}$. We have that $M = Lit_{P'}$ is trivially a model of $P'$. We can furthermore prove that $M$ is a minimal model. Indeed, let $M' \subset M$. Note that due to the definition of a model in ASP, we must either have that $M'$ is a consistent model or that $M' = Lit_P$, which cannot be the case since $M' \subset Lit_P$. Let $\pi'$ be defined as in the first part of this proof. We can then apply the same line of reasoning as in the first part of this proof where we show that $M$ is indeed a minimal model and hence an answer set of $P'$.
Clearly, since $M$ is an inconsistent answer set of $P'$, then due to the semantics of constraint rules we know that either $P$ is an inconsistent program (if $M$ violates no constraint rules in $C$) and thus has $Lit_P$ as the unique inconsistent answer set or $P$ has no answer sets (if $M$ violates some constraint rule in $C$).
Now assume that $\pi \in C_P \setminus C_{P'}$. We then know that there exists some $\pi'$ with $\pi' > \pi$ such that $\pi' \in S_{P'}$. As in the first part of this proof we obtain that $M' = \{l \mid N'(l) = 1, l \in Lit_{P'}\}$, with $N'$ the necessity measure induced by $\pi'$, is the unique answer set of $P'$. Because of the semantics of constraint rules we furthermore know that either $M'$ is the answer set of $P$ or that $P$ has no answer set (i.e. $M'$ violates some constraint rule in $C$).
We know by assumption that we obtain $\pi$, the vacuous distribution, from $\pi'$ by considering the constraints associated with the constraint rules in $C$. We furthermore know that for a rule $r = (\leftarrow l_1, ..., l_m)$ with $r \in C$ we must have that $\min(N'(l_1), ..., N'(l_m)) > 0$, as otherwise $\pi'$ would be a model of

$C$, i.e. we would be in the first case of this proof. Thus, it readily follows that $M'$ is not an answer set of $P$ because $M'$ violates some constraint $r \in C$, i.e. $P$ has no answer sets.

□

*Proposition 2*

Let $P$ be a simple program. If $M$ is an answer set of $P$ then the possibility distribution $\pi$ defined by $\pi(\omega) = 1$ iff $\omega \models M$ and $\pi(\omega) = 0$ otherwise belongs to $S_P$.

*Proof*

If $M$ is an answer set of $P$, then $M$ is by definition a model of $P$. If $M$ is consistent, then for every rule $r = (l_0 \leftarrow l_1, ..., l_m)$ with $r \in P$ we know that $l_0 \in M$ whenever $\{l_1, ..., l_m\} \subseteq M$. Otherwise, we know that $M = Lit_P$. Furthermore, due to Lemma 1 we know that defining $\pi(\omega) = 1$ if $\omega \models M$ and $\pi(\omega) = 0$ gives us $M = \{l \mid N(l) = 1, l \in Lit_P\}$. It is then easy to see that $\pi$ satisfies every constraint in $C_P$ and thus that $\pi \models C_P$.

We now show that $\pi$ is a minimally specific possibilistic model. To prove this, assume that this is not the case, i.e. $\pi \notin S_P$. This implies that there exists some other possibilistic model $\pi'$ such that $\pi' > \pi$ and in particular that there is some world $\omega$ such that $\pi'(\omega) > \pi(\omega) = 0$. By definition, $\pi(\omega) = 0$ if $\omega \not\models M$, i.e. $\pi(\omega) = 0$ if for some literal $l \in M$ we have that $\omega \not\models l$ or, equivalently, $\omega \models \neg l$. Then since $\pi'(\omega) > 0$, we find that $N'(l) < 1$ whereas $N(l) = 1$ due to the construction of $\pi$. Now let $M' = \{l \mid N'(l) = 1, l \in Lit_P\}$. It is easy to see that $M'$ is a model of $P$ since $\pi'$ is by assumption a possibilistic model, i.e. $\pi'$ satisfies the constraints $N'(l_0) \geq \min(N'(l_1), ..., N'(l_m))$ imposed by the rules $(l_0 \leftarrow l_1, ..., l_m) \in P$ and thus $l_0 \in M'$ whenever $\{l_1, ..., l_m\} \subseteq M'$ due to the construction of $M'$. However, since $\pi' > \pi$ we know that $M' \subseteq M$ and due to $N'(l) < 1$ and $N(l) = 1$ for some $l \in M$ we know that $M' \subset M$. Thus we find that $M$ is not a minimal model and therefore that $M$ is not an answer set, which is a contradiction. □

*Proposition 3*

Let $P$ be a disjunctive program, $V$ a valuation and let $\pi \in S^{\mathrm{s}}_{(P,V)}$ be such that

$$\forall l \in Lit_P \cdot V(l) = N(l) \text{ ; and} \tag{1}$$

$$\forall l \in Lit_P \cdot N(l) \in \{0, 1\} \tag{2}$$

then $M = \{l \mid N(l) = 1, l \in Lit_P\}$ is an answer set of the disjunctive program $P$.

*Proof*

We need to prove, when $M$ is consistent, that $M$ is a minimal model of the positive disjunctive program $P^M$. Consider a rule $r \in P$ with $r = (l_0; ...; l_k \leftarrow l_{k+1}, ..., l_m, \mathit{not}\ l_{m+1}, ..., \mathit{not}\ l_n)$. We know from Definition 6 that $\pi \in S^{\mathrm{s}}_{(P,V)}$ satisfies the constraint

$$\max(N(l_0), ..., N(l_k)) \geq \min(N(l_{k+1}), ..., N(l_m), 1 - V(l_{m+1}), ..., 1 - V(l_n)). \tag{3}$$

Note that due to (1) and (2) we know that $V(l_{m+1}), ..., V(l_n)$ all belong to $\{0, 1\}$. Moreover, because we use the minimum, as soon as $V(l_i) = 1$ and thus $(1 - V(l_i)) = 0$ for some $i \in \{m+1, ..., n\}$, the constraint (3) becomes trivial. Indeed, the constraint becomes $\max(N(l_0), ..., N(l_k)) \geq 0$. Correspondingly we know that in that case we have $V(l_i) = 1$ or, equivalently, $N(l_i) = 1$ and thus that $l_i \in M$ per definition of $M$. Thus the rule $r$ will be completely omitted from the reduct $P^M$. Otherwise, when $V(l_{m+1}) = ... = V(l_n) = 0$, the constraint simplifies to

$$\max(N(l_0), ..., N(l_k)) \geq \min(N(l_{k+1}), ..., N(l_m)) \tag{4}$$

in which case the reduct $P^M$ will contain the rule $(l_0; ...; l_k \leftarrow l_{k+1}, ..., l_m)$. Also, continuing in the same line of reasoning, we find that $C^{s}_{P^M} = C^{s}_{(P,V)}$ and $S^{s}_{P^M} = S^{s}_{(P,V)}$.

We can then verify that $M$ is a minimal model of $P^M$. In the same line of reasoning as in the proof of Proposition 1, we can show that $M$ is a model of $P^M$. Specifically, we now have that the constraint imposed by a rule ensures that $N(l_i) = 1$ for some $l_i$ with $0 \leq i \leq k$. Assuming that $M$ is a consistent model, we can use the same line of reasoning as in the proof of Proposition 1 to show that $M$ is a minimal model of $P^M$.

Finally, we need to ensure that $Lit_P$ is the unique answer set of $P$ if $P$ has no consistent answer sets. This implies that $M$ is inconsistent, as otherwise we would be in the case mentioned above. Inconsistencies can only arise since either $N(\bot) = 1$, i.e. because a constraint was violated, or $N(l) = 1$ and $N(\neg l) = 1$ with $l \in Lit_P$, i.e. because the program has two inconsistent conclusions. This is due to the constraints induced by $P$ and due to (2), from which we know that these necessity degrees can only be 1 (if they were 0, they would not cause inconsistencies). Furthermore, stating that $l \wedge \neg l \equiv \bot$. As such, we know that for some $l \in Lit_P$ we have that $\Pi(\neg l) = \Pi(l) = 0$. By definition of the possibility measure $\Pi$ this means that for every $\omega \in \Omega$ we have that $\pi(\omega) = 0$. This can only be the case if $S^{s}_{(P,V)}$ is a singleton, since for every other possibility distribution $\pi' \neq \pi$ we have that $\pi' < \pi$. We thus find that $S^{s}_{(P,V)} = \{\pi\}$ and that $\forall l \in Lit_P \cdot N(l) = 1$, i.e. $M = Lit_P$. □

*Proposition 4*
Let $P$ be a disjunctive program. If $M$ is an answer set of $P$, there is a valuation $V$, defined as $V(l) = 1$ if $l \in M$ and $V(l) = 0$ otherwise, and a possibility distribution $\pi$, defined as $\pi(\omega) = 1$ if $\omega \models M$ and $\pi(\omega) = 0$ otherwise, such that $\pi \in S^{s}_{(P,V)}$ and for every $l \in Lit_P$ we have $V(l) = N(l)$.

*Proof*
When $M$ is consistent, it readily follows from Lemma 1 that $N(l) = 1$ if $l \in M$ and $N(l) = 0$ otherwise. If $M$ is inconsistent, i.e. if $M = Lit_P$, then for every $\omega$ we have $\pi(\omega) = 0$ since there does not exist $\omega \models Lit_P$, i.e. for every $l \in Lit_P$ we have $N(l) = 1$. Hence in both cases we find that $V(l) = N(l)$.

We now show that $\pi \in S^{s}_{(P,V)}$. We start by showing that $C^{s}_{P^M} = C^{s}_{(P,V)}$. Since $M$ is an answer set of the disjunctive program $P$, it is also a minimal model of the reduct $P^M$. This reduct is obtained by considering the rules $r \in P$ which are of

the form $(l_0; ...; l_k \leftarrow l_{k+1}, ..., l_m, not\ l_{m+1}, ..., not\ l_n)$. The corresponding constraint $\gamma_V(r)$ in $C_{(P,V)}$ is then

$$\max(N(l_0), ..., N(l_k)) \geq \min(N(l_1), ..., N(l_m), 1 - V(l_{m+1}), ..., 1 - V(l_n)).$$

For every rule $r \in P$ we have $r' \in P^M$ with $r' = (l_1; ...; l_k \leftarrow l_{k+1}, ..., l_m)$ whenever $\{l_{m+1}, ..., l_n\} \cap M = \emptyset$. Notice that this implies that $V(l_{m+1}) = ... = V(l_n) = 0$ due to how we defined $V$ and thus we obtain

$$\max(N(l_0), ..., N(l_k)) \geq \min(N(l_{k+1}), ..., N(l_m))$$

which corresponds exactly to the constraint induced by $r' \in P^M$. Otherwise, whenever $\{l_{m+1}, ..., l_n\} \cap M \neq \emptyset$ we have that $r$ has no counterpart in $P^M$. Similarly, the constraint then reduces to the form $\max(N(l_0), ..., N(l_k)) \geq 0$, which is trivially true. We thus find that $C_{P^M} = C_{(P,V)}$ and $S_{P^M} = S_{(P,V)}$.

It now readily follows that $\pi$ is a possibilistic model of $P^M$. Indeed, for every constraint

$$\max(N(l_0), ..., N(l_k)) \geq \min(N(l_{k+1}), ..., N(l_m))$$

imposed by a rule $(l_0; ...; l_k \leftarrow l_{k+1}, ..., l_m) \in P^M$ we have that there exists some $l_i \in M$ with $0 \leq i \leq k$ whenever $\{l_{k+1}, ..., l_m\} \subseteq M$. Otherwise $M$ would not be a model of $P^M$ and then $M$ would certainly not be an answer set. Due to the construction of $\pi$, where $N(l) = 1$ whenever $l \in M$, it readily follows that $\pi$ satisfies every constraint in $C^{\mathrm{s}}_{P^M}$, i.e. $\pi$ is a possibilistic model of $P^M$. Similar as in the proof of Proposition 2, we can then verify that $\pi$ is indeed a minimally specific possibilistic model. $\square$

*Proposition 5*

Let $P$ be a possibilistic positive clausal program without possibilistic constraint rules. Then $P^\star_{\mathrm{w}}$ is a possibilistic answer set of $P$.

*Proof*

We need to prove that $P^\star_{\mathrm{w}}$ is a possibilistic answer set of $P$, or, equivalently, that the minimally specific possibility distribution $\pi$ encoded by the set of constraints $\{N(e) \geq \lambda \mid e^\lambda \in P^\star_{\mathrm{w}}\}$ is a possibilistic answer set of $P$.

To see this, recall that for every possibilistic rule $p \in P$ of the form $p = (r, \lambda)$ with $r = (e_0 \leftarrow e_1, ..., e_m)$ we know from Definition 10 that we have the corresponding constraint $N(e_0) \geq \lambda'$ in $C^{\mathrm{w}}_P$ with $\lambda' = \min(N(e_1), ..., N(e_m), \lambda)$. We obtained $P^\star_{\mathrm{w}}$ by repeatedly applying the operator $T^{\mathrm{w}}_P$ as defined in Definition 13, starting from the minimal clausal valuation $V = \emptyset$, until the fixpoint is reached. As such, we know that when ${e_0}^{\lambda''} \in P^\star_{\mathrm{w}}$ this implies that $\exists r \in P_{\lambda''}$ such that $\forall i \in 1, ..., m \cdot (P^\star_{\mathrm{w}})^{\lambda''} \models e_i$.

We then have that $\lambda'' = \lambda'$. Indeed, assume that $\lambda'' < \lambda'$. This would imply that either $r \notin P_{\lambda'}$ or that $\exists i \in 1, ..., m \cdot (P^\star_{\mathrm{w}})^{\lambda'} \not\models e_i$. The first cannot be the case since this would imply that $p = (r, \lambda) \in P$ with $\lambda < \lambda'$, i.e. $\lambda' \neq \min(N(e_1), ..., N(e_m), \lambda)$. Similarly, the latter cannot be the case since then $\min(N(e_1), ..., N(e_m)) < \lambda'$. A similar line of reasoning can be used to verify that we do not have that $\lambda'' > \lambda'$ as this would imply that $P^\star_{\mathrm{w}}$ is not a least fixpoint.

Since we have that $\lambda' = \lambda''$ this implies that the constraints imposed by $P^\star_{\mathrm{w}}$ and $C^{\mathrm{w}}_P$ are the same. Hence also their minimally specific possibility distributions are the same. Thus we find that $\pi \in S^{\mathrm{w}}_P$. $\square$

*Proposition 6*
A valuation $E$ is a possibilistic answer set of the possibilistic clausal program $P$ without possibilistic constraint rules iff $E$ is a possibilistic answer set of $P^E$.

*Proof*
($\Rightarrow$) Let the valuation $E$ be a possibilistic answer set of $P$ and $\pi$ the corresponding possibility distribution such that $E = \left\{e^{N(e)} \mid e \in \mathit{Clause}_P\right\}$. Furthermore, we choose a $V$ such that $V(e) = N(e)$. From Definition 11 we know that $\pi \in S^{\mathrm{w}}_{(P,\pi_V)}$ since $E$ is a possibilistic answer set of $P$. Let us now consider any possibilistic rule $p \in P$ with $p = (r, \lambda)$, $r = (e_0 \leftarrow e_1, ..., e_m, \mathit{not}\ e_{m+1}, ..., \mathit{not}\ e_n)$ and $\lambda \in ]0, 1]$. We know from Definition 10 that $\pi$ satisfies the constraint

$$N(e_0) \geq \min(N(e_1), ..., N(e_m), 1 - V(e_{m+1}), ..., 1 - V(e_n), \lambda). \tag{5}$$

This constraint either reduces to the trivial constraint $N(e_0) \geq 0$ (whenever $V(e_{m+1}) = 1$ or ... or $V(e_n) = 1$) or it simplifies to

$$N(e_0) \geq \min(N(e_1), ..., N(e_m), \lambda') \tag{6}$$

with $\lambda' = \min(1 - V(e_{m+1}), ..., 1 - V(e_n), \lambda)$. Note that we can also write $\lambda'$ as $\lambda' = \min(\lambda_{body}, \lambda_{rule})$ with $\lambda = \lambda_{rule}$ and $\lambda_{body} = 1 - \max(V(e_{m+1}), ..., V(e_n))$. Hence we find from Definition 14 that the reduct $P^E$ will contain the rule $((e_0 \leftarrow e_1, ..., e_m), \lambda')$. In the same line of reasoning we find that $C^{\mathrm{w}}_{P^E} = C^{\mathrm{w}}_{(P,\pi_V)}$ and $S^{\mathrm{w}}_{P^E} = S^{\mathrm{w}}_{(P,\pi_V)}$. Hence we find that $E$ is also a possibilistic answer set of $P^E$ since $\pi \in S^{\mathrm{w}}_{P^E}$.
($\Leftarrow$) Let the valuation $E$ be a possibilistic answer set of $P^E$ and $\pi$ the corresponding possibility distribution such that $E = \left\{e^{N(e)} \mid e \in \mathit{Clause}_P\right\}$. Furthermore, we choose a $V$ such that $V(e) = N(e)$. We now follow a similar line of reasoning as before. Indeed, we know from Definition 10 that $\pi$ satisfies the constraints (6) induced by the rules in $P^E$. By definition of the reduct from Definition 14 we know that the rules in $P^E$ are obtained from a corresponding program $P$ consisting of rules of the form $p = (r, \lambda)$ with $r = (e_0 \leftarrow e_1, ..., e_m, \mathit{not}\ e_{m+1}, ..., \mathit{not}\ e_n)$, each of which induces the constraint (5). Specifically, due to the definition of the reduct operator, we know that the rule $p' = (r', \lambda') \in P^E$ corresponds with a rule $p = (r, \lambda) \in P$ such that $\lambda' = \min(1 - V(e_{m+1}), ..., 1 - V(e_n), \lambda)$ and for which we know that $V(e_{m+1}) \neq 1$ and ... and $V(e_n) \neq 1$. For all other rules in $P$ that do not correspond with a rule in $P^E$ we know from Definition 14 that $N(e_0) \geq 0$, i.e. the rule encode trivial information and can be ignored. As such we again find that $C^{\mathrm{w}}_{P^E} = C^{\mathrm{w}}_{(P,\pi_V)}$ and $S^{\mathrm{w}}_{P^E} = S^{\mathrm{w}}_{(P,\pi_V)}$. Hence we find that $E$ is also a possibilistic answer set of $P$ since $\pi \in S^{\mathrm{w}}_P$. $\square$

*Proposition 7* (*possibilistic normal program; brave reasoning*)
Let $P$ be a possibilistic normal program. The problem of deciding whether there exists a possibilistic answer set $V$ of $P$ such that $V(l) \geq \lambda$ is NP-complete.

*Proof*
(membership) Notice that the reduct defined in Definition 14 can also be applied to possibilistic normal programs. Indeed, possibilistic normal programs are a special cases of possibilistic clausal programs where every clause consists of exactly one literal. Since possibilistic normal programs are a special case, it readily follows from previous proofs that we can use this syntactic method to find possibilistic answer sets of possibilistic normal programs. Furthermore, when considering possibilistic normal program, we can simplify the reduct. We can write $\forall i \in \{m+1,...,n\} \cdot e_i \notin V^{\underline{1-\lambda}}$ instead of $\forall i \in \{m+1,...,n\} \cdot V^{\underline{1-\lambda}} \not\models e_i$, i.e. the reduct $P^V$ with $P$ a possibilistic normal program can be determined in polynomial time.

To determine whether $V(l) \geq \lambda$ with $V$ a possibilistic answer set we need to guess a valuation $V$ such that $V(l) \geq \lambda$. Given such a non-deterministic guess, we can determine the reduct $P^V$ in polynomial time. We can then verify in polynomial time using the immediate consequence operator $T_{P^V}$ from Definition 13 whether $V$ is indeed a possibilistic answer set of $P^V$ and thus a possibilistic answer set of $P$. Indeed, since we are dealing with literals we can simplify $V^\lambda \models e_i$ to $e_i \in V^\lambda$ to make this operator polynomial, similar as how we did for the reduct from Definition 14. Hence determining whether $V(l) \geq \lambda$ with $V$ a possibilistic answer set is an NP problem.
(hardness) We reduce the problem of determining the satisfiability of a QBF of the form $\phi = \exists X \cdot p(X)$ with $p(X)$ in DNF, i.e. of the form $\theta_1 \vee ... \vee \theta_n$ with each $\theta_i$ a conjunction of literals, to the problem of deciding whether there exists a possibilistic answer set $V$ such that $V(l) \geq \lambda$. We define the possibilistic normal program $P_\phi$ corresponding to $\phi$ as

$$P_\phi = \{\mathbf{1\colon}\ x \leftarrow \mathit{not}\ \neg x \mid x \in X\} \cup \{\mathbf{1\colon}\ \neg x \leftarrow \mathit{not}\ x \mid x \in X\} \tag{7}$$
$$\cup \{\mathbf{1\colon}\ \mathit{sat} \leftarrow \theta_t \mid 1 \leq t \leq n\} \tag{8}$$

where we identify the conjunction of literals $\theta_t$ in (8) with a set of literals. It readily follows that the QBF is satisfiable if and only if $V(\mathit{sat}) = 1$. Indeed, the rules in (7) generate as many possibilistic answer sets as there are interpretations of $X$. The rules from (8) ensure that '*sat*' is contained in the possibilistic answer set whenever for a chosen interpretation of $X$ it holds that $p(X)$ is satisfiable. It readily follows from the construction of $P_\phi$ that $N(\mathit{sat}) = 1$. Hence we have reduced the boolean satisfiability problem to the problem of determining whether there exists a possibilistic answer set $V$ such that $V(\mathit{sat}) = 1$. □

*Proposition 8* (*possibilistic normal program; cautious reasoning*)
Let $P$ be a possibilistic normal program. The problem of deciding whether for all possibilistic answer sets $V$ of $P$ we have that $V(l) \geq \lambda$ is coNP-complete.

*Proof*
(membership) We show that the complementary problem is in NP. To determine whether there exists a possibilistic answer set $V$ with $V(l) < \lambda$, we guess such a valuation $V$. Given this non-deterministic guess, we can determine the reduct $P^V$ in polynomial time (where we take $P^V$ as discussed in Proposition 9). We can then verify in polynomial time using the immediate consequence operator $T_{P^V}$ from Definition 13 (simplified as in the proof of Proposition 9) whether $V$ is indeed a possibilistic answer set of $P^V$ and thus a possibilistic answer set of $P$. Hence determining whether there exists a possibilistic answer set $V$ such that $V(l) < \lambda$ is a problem in NP. Deciding whether for all possibilistic answer sets $V$ we have that $V(l) \geq \lambda$ is thus in coNP.
(hardness) Analogous to the hardness proof in Proposition 9 where we now solve a QBF of the form $\phi = \forall X \cdot p(X)$ and where we are interested in whether for all possibilistic answer sets $V$ we have that $V(sat) = 1$. In particular, the possibilistic answer sets of $P$ are exactly the models of the proposed SAT problem (or QBF). Hence the problem described in this proposition corresponds with the problem of entailment checking. □

*Proposition 9* (*possibilistic disjunctive program; brave reasoning*)
Let $P$ be a possibilistic disjunctive program. The problem of deciding whether there is a possibilistic answer set $V$ such that $V(l) \geq \lambda$ is a $\Sigma_2^{\mathsf{P}}$-complete problem.

*Proof*
(membership) We discussed in the proof of Proposition 9 how the reduct defined in Definition 14 can also be applied to possibilistic normal programs. In addition, notice that the reduct only affects the body of the rule. As such, we can also apply the reduct (where we consider literals instead of clauses, which ensures that the reduct can be determined in polynomial time) to a possibilistic disjunctive program to obtain a possibilistic positive disjunctive program. Furthermore, because the reduct only affects the body, it is easy to see that this syntactic method is also correct for possibilistic disjunctive programs (i.e. the possibilistic answer sets obtained through the syntactic method corresponds perfectly with the semantical definition from Definition 7). Indeed, in the proof of Proposition 8 we then have that (5) becomes $\max(N(l_0), ..., N(l_k)) \geq \min(N(l_{k+1}), ..., N(l_m), 1 - V(l_{m+1}), ..., 1 - V(l_n), \lambda)$ whereas (6) becomes $\max(N(l_0), ..., N(l_k)) \geq \min(N(e_{k+1}), ..., N(e_m), \lambda)$. As such, we can verify that indeed $S^{\mathsf{s}}_{P^V} = S^{\mathsf{s}}_{(P,V)}$. We can thus prove correctness of this syntactic approach following a similar line of reasoning as in Proposition 8.

To determine whether there is a possibilistic answer set $V$ such that $V(l) \geq \lambda$ we need to guess a valuation $V$ such that $V(l) \geq \lambda$. Given such a non-deterministic guess, we can determine the reduct $P^V$ in polynomial time. Since $P^V$ is a possibilistic positive disjunctive program, we know that $P^V$ does not necessarily have a

unique possibilistic answer set. We can show that $V$ is not an answer set by guessing a $V'$ such that $V' \subset V$ with $V'$ a model of $P^V$. Thus, to verify in constant time whether $V$ is a possibilistic answer set of the possibilistic positive disjunctive program $P^V$, we can rely on an NP-oracle. Thus, determining whether there is a possibilistic answer set $V$ of a possibilistic disjunctive program such that $V(l) \geq \lambda$ is in $\mathsf{NP}^{\mathsf{NP}}$, i.e. in $\Sigma_2^{\mathsf{P}}$.

(hardness) We reduce the problem of determining the satisfiability of a QBF of the form $\phi = \exists X_1 \forall X_2 \cdot p(X_1, X_2)$ with $p(X_1, X_2)$ in DNF, i.e. of the form $\theta_1 \vee ... \vee \theta_n$ with each $\theta_i$ a conjunction of literals, to the problem of deciding whether there exists a possibilistic answer set $V$ of a possibilistic disjunctive program such that $V(l) \geq \lambda$. We define the possibilistic disjunctive program $P_\phi$ corresponding to $\phi$ as

$$\begin{aligned} P_\phi = &\{\mathbf{1:}\ x; x' \leftarrow \ \mid x \in (X_1 \cup X_2)\} & (9)\\ &\cup \{\mathbf{1:}\ sat \leftarrow \theta'_t \mid 1 \leq t \leq n\} & (10)\\ &\cup \{\mathbf{1:}\ x \leftarrow sat \mid x \in X_2\} \cup \{\mathbf{1:}\ x' \leftarrow sat \mid x \in X_2\} & (11) \end{aligned}$$

where we identify the conjunction of literals $\theta'_t$ in (10) with a set of literals and where we replace occurrences of negated atoms of the form $\neg x$ with fresh atoms $x'$.

It readily follows that the QBF is satisfiable if and only if $V(sat) = 1$. Indeed, the rules in (9) generate as many possibilistic answer sets as there are interpretations of $X_1$ and $X_2$. The rules from (10) ensure that '*sat*' is contained in the possibilistic answer set whenever, for a chosen interpretation of $X_1$ and $X_2$, it holds that $p(X_1, X_2)$ is satisfiable. It readily follows from the construction of $P_\phi$ that $N(sat) = 1$. The rules in (11) then employ saturation to ensure that it holds for every interpretation of $X_2$. Indeed, assume that for some interpretation of $X_1$ and some interpretation of $X_2$ it holds that $p(X_1, X_2)$ is satisfiable, but not for some other interpretation of $X_2$. In particular, assume that the first interpretation gives rise to the possibility distribution $\pi_{\text{sat}}$ and the latter to the possibility distribution $\pi_{\text{notsat}}$. Then, clearly, $N_{\text{notsat}}(sat) = 0$. Furthermore, since an interpretation of $X_2$ is a strict subset of $X_2$ due to (9), we know that due to the rules in (11) that $\forall \omega \cdot \pi_{\text{notsat}}(\omega) \leq \pi_{\text{sat}}(\omega)$ and in particular that $\exists \omega \cdot \pi_{\text{notsat}}(\omega) < \pi_{\text{sat}}(\omega)$, i.e. $\pi_{\text{sat}}$ is not a least specific possibility distribution and would not give rise to a possibilistic answer set. Thus, if $p(X_1, X_2)$ did not hold for every interpretation of $X_2$ we would not have that $N(sat) = 1$. □

*Proposition 10* (*possibilistic disjunctive program; cautious reasoning*)
Let $P$ be a possibilistic disjunctive program. The problem of deciding whether for all possibilistic answer sets $V$ we have that $V(l) \geq \lambda$ is a $\Pi_2^{\mathsf{P}}$-complete problem.

*Proof*
(membership) Take $P' = P \cup \{\mathbf{1:}\ l' \leftarrow not\ l\}$. An answer set $V'$ of $P'$ exists with $V'(l) > 1 - \lambda$ iff we do not have for all answer sets $V$ of $P$ that $V(l) \geq \lambda$. As such, this is the complementary problem of Proposition 11 and thus in in $\Sigma_2^{\mathsf{P}}$.
(hardness) We reduce the problem of determining the satisfiability of a QBF of the form $\phi = \forall X_1 \exists X_2 \cdot p(X_1, X_2)$ with $p(X_1, X_2)$ in CNF, i.e. of the form $\theta_1 \wedge ... \wedge \theta_n$

with each $\theta_i$ a disjunction of literals, to the problem of deciding whether for all possibilistic answer sets $V$ of a possibilistic disjunctive program we have that $V(l) \geq \lambda$. We define the possibilistic disjunctive program $P_\phi$ corresponding to $\phi$ as

$$
\begin{aligned}
P_\phi = &\{\mathbf{1}\!:\ x; x' \leftarrow\ \mid x \in (X_1 \cup X_2)\} & (12)\\
&\cup \{\mathbf{1}\!:\ \mathit{unsat} \leftarrow \theta'_t \mid 1 \leq t \leq n\} & (13)\\
&\cup \{\mathbf{1}\!:\ x \leftarrow \mathit{unsat} \mid x \in X_2\} \cup \{\mathbf{1}\!:\ x' \leftarrow \mathit{unsat} \mid x \in X_2\} & (14)\\
&\cup \{\mathbf{1}\!:\ \mathit{sat} \leftarrow \mathit{not}\ \mathit{unsat}\} & (15)
\end{aligned}
$$

where $\theta'_t$ in (13) is obtained by taking the negation of $\theta_t$, i.e. if $\theta_t$ is the disjunction $x_{11} \vee x_{21} \vee \neg x_{12}$ then $\theta'_t$ is the conjunction $x'_{11} \wedge x'_{21} \wedge x_{12}$. Furthermore, we identify the resulting conjunction of literals with a set of literals and we replace occurrences of negated atoms of the form $\neg x$ with fresh atoms $x'$.

It readily follows that the QBF is satisfiable if and only if $V(\mathit{sat}) = 1$. Indeed, the rules in (12) generate as many possibilistic answer sets as there are interpretations of $X_1$ and $X_2$. The rules from (13) ensure that '*unsat*' is contained in the possibilistic answer set whenever, for a chosen interpretation of $X_1$ and $X_2$, it holds that $p(X_1, X_2)$ is unsatisfiable. It readily follows from the construction of $P_\phi$ that $N(\mathit{unsat}) = 1$. The rules in (14) then employ saturation to ensure that $p(X_1, X_2)$ is unsatisfiable for every interpretation of $X_2$. Indeed, assume that for some interpretation of $X_1$ and some interpretation of $X_2$ it holds that $p(X_1, X_2)$ is unsatisfiable, but that there is some other interpretation of $X_2$ such that $p(X_1, X_2)$ is satisfiable. In particular, assume that the first interpretation gives rise to the possibility distribution $\pi_{\text{unsat}}$ and the latter to the possibility distribution $\pi_{\text{sat}}$. Then, clearly, $N_{\text{sat}}(\mathit{unsat}) = 0$. Furthermore, since an interpretation of $X_2$ is a strict subset of $X_2$ due to (12), we know that due to the rules in (14) that $\exists \omega \cdot \pi_{\text{sat}}(\omega) \leq \pi_{\text{unsat}}(\omega)$ and in particular that $\exists \omega \cdot \pi_{\text{sat}}(\omega) < \pi_{\text{unsat}}(\omega)$, i.e. $\pi_{\text{unsat}}$ is not a least specific possibility distribution and would not give rise to a possibilistic answer set. Finally, due to (15) we know that $N(\mathit{sat}) = 1$ whenever $N(\mathit{unsat}) = 0$. Thus, if $p(X_1, X_2)$ was unsatisfiable for all interpretations of $X_2$ for some interpretation of $X_1$ we would not have that $N(\mathit{sat}) = 1$. □

*Proposition 11* (*weak disjunction, positive clausal program; brave reasoning*)
Let $P$ be a positive clausal program. The problem of deciding whether a clause '$e$' is entailed by a consistent answer set $E$ of $P$ is $\mathsf{BH}_2$-hard.

*Proof*
It readily follows from Lemma 2 that when $M$ is the answer set of $P$ we have that $M$ is unique up to logical equivalence. It may however be that $P$ does not have a consistent answer set. For instance, $P = \{(a \leftarrow), (\neg a \leftarrow)\}$ does not have a consistent answer set.
To prove hardness, i.e. to prove that we can solve $\mathsf{BH}_2$-complete problems using brave reasoning over positive clausal programs, we show that the sat-unsat problem can be modelled using positive clausal programs. Sat-unsat is the canonical

$\mathsf{BH}_2$-complete problem and consists of determining for some pair $(T, S)$ of propositional theories in conjunctive normal form (CNF) whether $T$ is satisfiable and $S$ is unsatisfiable. We can see the propositional theory $T$ as a formula of the form

$$\phi = (k_{11} \vee \ldots \vee k_{1i_1}) \wedge (k_{21} \vee \ldots \vee k_{2i_2}) \wedge \ldots \wedge (k_{n1} \vee \ldots \vee k_{ni_n})$$

and the propositional theory $S$ as a formula of the form

$$\psi = (s_{11} \vee \ldots \vee s_{1j_1}) \wedge (s_{21} \vee \ldots \vee s_{2j_2}) \wedge \ldots \wedge (s_{m1} \vee \ldots \vee s_{mj_m})$$

where $k_{ij}$ and $s_{ij}$ are literals such that none of the literals used in $\phi$ occur in $\psi$ and vice versa. The positive clausal program $P = P_1 \cup P_2$ that can be used to solve the sat-unsat problem contains the set of rules $P_1$:

$$\begin{aligned} k_{11} \vee \ldots \vee k_{1i_1} &\leftarrow \\ k_{21} \vee \ldots \vee k_{2i_2} &\leftarrow \\ &\vdots \\ k_{n1} \vee \ldots \vee k_{ni_n} &\leftarrow \end{aligned}$$

and the set of rules $P_2$:

$$\begin{aligned} unsat \vee s_{11} \vee \ldots \vee s_{1j_1} &\leftarrow \\ unsat \vee s_{21} \vee \ldots \vee s_{2j_2} &\leftarrow \\ &\vdots \\ unsat \vee s_{m1} \vee \ldots \vee s_{mj_m} &\leftarrow . \end{aligned}$$

The rules in $P_1$ are used to determine whether $T$ is satisfiable. Indeed, since an answer set $M \neq Clause_P$ of $P$ must, by definition, be consistent, it readily follows that whenever $P$ has a consistent answer set $M$ we must have that the formula $\phi$ is satisfiable. The rules in $P_2$ are used to verify whether $S$ is unsatisfiable. Notice that we will only be able to derive '*unsat*' from $P$ if and only if $S$ is unsatisfiable. Indeed, '*unsat*' can only be derived from an answer set $M$ if '*unsat*' is true in every model of program $P$. If $S$ were satisfiable, we could always take a model of $S$, which would automatically be a model of program $P_2$ in which '*unsat*' is false, thus preventing us from deriving '*unsat*'. Hence we find that there exists a consistent answer set $M$ of the positive clausal program $P$ such that $M \models unsat$ iff $T$ is satisfiable and $S$ is unsatisfiable. □

*Proposition 12* (*weak disjunction, positive clausal program; brave reasoning*)
Let $P$ be a positive clausal program. The problem of deciding whether a clause '$e$' is entailed by a consistent answer set $M$ of $P$ is in $\mathsf{BH}_2$.

*Proof*
We translate the problem of deciding whether '$e$' is entailed by a consistent answer set $M$ of the positive clausal program $P$ to the problem of consistency and entailment checking in meta-epistemic logic (MEL) (Banerjee and Dubois 2009). MEL corresponds to a fragment of KD modal logic (Huth and Ryan 2004) where nesting

of propositional formulas and modalities is not allowed (i.e. the depth of modal operators is limited to exactly 1).

Let $\mathcal{V} = 2^{\mathcal{B}_P}$ be the set of all interpretations, where each interpretation $w \in \mathcal{V}$ is defined as a mapping $w : \mathcal{B}_P \to \{0, 1\}$. For a formula $\phi$ in propositional logic, $w \models \phi$ indicates that $w$ satisfies $\phi$, i.e. that $w$ is a model of $\phi$. The set of models of a propositional formula $\phi$ is denoted by $[\phi] = \{w \mid w \models \phi\}$. The epistemic state of an agent $\mathcal{E}$ is represented by $K \subseteq \mathcal{V}$. We have $K \models \Box\phi$ iff $K \subseteq [\phi]$, $K \models \neg\phi$ iff $K \not\models \phi$, $K \models \phi \wedge \psi$ iff $K \models \phi$ and $K \models \psi$ and we have $\vee$ defined in the usual way, i.e. $\phi \vee \psi := \neg(\neg\phi \wedge \neg\psi)$. The models of MEL-formulae are called meta-models to avoid confusion with the models of propositional formulae.
For every $r \in P$, where $r$ is of the form

$$e_0 \leftarrow e_1, ..., e_m \tag{16}$$

with $e_i$ clauses for $0 \leq i \leq m$, we add the MEL-formula

$$\neg\Box(e_1 \wedge ... \wedge e_m) \vee \Box e_0. \tag{17}$$

to the MEL theory $\mathcal{K}$. What this tells us is that either $e_1 \wedge ... \wedge e_m$ is not entailed by $K$ or, that $e_0$ is entailed by $K$. We now show that every meta-model $K$ of the MEL theory $\mathcal{K}$ corresponds with a possibilistic model $\pi$ of $P$ iff $P$ has consistent models, which is because $N(e_i) = 1$ iff $K \models \Box(e_i)$. Let $K$ be a meta-model of the MEL theory $\mathcal{K}$ and let $\pi$ be defined as $\pi(\omega) = 1$ if $\omega \in K$ and $\pi(\omega) = 0$ otherwise. For a rule of the form (16) it can readily be seen that $\pi$ is a possibilistic model. Indeed, assume that $N(e_1) = ... = N(e_m) = 1$. This implies that for every world $\omega$ such that $\omega \models \neg e_1 \vee ... \vee \neg e_m$ we have that $\pi(\omega) = 0$. Hence, for every $\omega$ such that $\pi(\omega) = 1$ we must have that $e_0$ is satisfied in $\omega$ as otherwise the MEL-formula (17) is not satisfied, i.e. we must have $N(e_0) = 1$. When we do not have that $N(e_1) = ... = N(e_m) = 1$ then the constraint $N(e_0) \geq \min(N(e_1), ..., N(e_m))$ is vacantly satisfied. It can also easily be seen that every meta-model corresponds with exactly one possibilistic model given the construction. It readily follows that for $\pi$ a possibilistic model of $P$ we have that $K = \{\omega \mid \pi(\omega) = 1\}$ is also a meta-model of $\mathcal{K}$ using a similar line of reasoning, given that $P$ is a consistent program.

Due to the correspondence between meta-models and possibilistic models, we have that a possibilistic model corresponding with a consistent answer set only exists if the associated MEL-theory $\mathcal{K}$ is satisfiable. From Lemma 2 we also know that the clause $e$ is entailed by the answer set of $P$ iff for every possibilistic model $\pi$ of $P$ we have that $N(e) = 1$, as otherwise we would not have for $\pi \in S_P^{\text{w}}$ that $N(e) = 1$. Hence we know that $e$ is entailed by an answer set of $P$ if $K \models \Box e$ for every meta-model $K$ of $\mathcal{K}$. A clause '$e$' thus belongs to a consistent answer set $M$ of $P$ if $\mathcal{K}$ is satisfiable and for every meta-model $K$ of $\mathcal{K}$ it holds that $K \models \Box e$. As satisfiability and entailment in KD for a modal depth of 1 are in $\mathsf{NP}$ and $\mathsf{coNP}$ respectively (Nguyen 2005), this concludes the proof. □

*Corollary 1* (*weak disjunction, positive clausal program; answer set existence*)
Determining whether a positive clausal program $P$ has a consistent answer set is an NP-complete problem.

*Proof*
The problem of determining whether a positive clausal program $P$ has an answer set reduces to the problem of satisfiability checking in MEL as in the proof of Proposition 14, which is a problem in NP. Furthermore, from the proof of Proposition 13 we know that satisfiability of a propositional theory can be checked by verifying whether a program $P$ has an answer set, hence this problem is also NP-hard. □

*Corollary 2* (*weak disjunction, positive clausal program; cautious reasoning*)
Cautious reasoning, i.e. determining whether a clause '$e$' is entailed by every answer set $M$ of a positive clausal program $P$ is coNP-complete.

*Proof*
This problem reduces to the problem of entailment checking in MEL as in the proof of Proposition 14, which is a problem in coNP. Furthermore, from the proof of Proposition 13 we know that unsatisfiability of a propositional theory can be checked by verifying whether some clause '$e$' (in particular, '*unsat*' in Proposition 13) is entailed by the answer sets of a positive clausal program $P$, hence this problem is also coNP-hard. □

*Proposition 13*
Let $P$ be a positive clausal program without classical negation. We can find the unique answer set of $P$ in polynomial time.

*Proof*
Applying the simplified immediate consequence operator can be done in polynomial time. Furthermore, only a polynomial number of applications of the operator are necessary since it is never possible to derive more information than the union of all the heads of all the rules and because after each application we either obtain at least one new clause or we have found an answer set. □

*Proposition 14* (*weak disjunction; brave reasoning*)
Let $P$ be a clausal program. The problem of deciding whether a clause '$e$' is entailed by a consistent answer set $M$ of $P$ is $\Sigma_2^{\mathsf{P}}$-hard.

*Proof*
We reduce the problem of determining the satisfiability of a QBF of the form $\phi = \exists X_1 \forall X_2 \cdot p(X_1, X_2)$ with $p(X_1, X_2)$ in DNF to the problem of deciding whether a clause '$e$' is entailed by a consistent answer set $M$ of $P$. Since the problem of determining satisfiability of QBFs of that form is the canonical $\Sigma_2^{\mathsf{P}}$-complete problem, this shows that the problem of deciding whether a clause '$e$' is entailed by a consistent answer set $M$ of $P$ is indeed $\Sigma_2^{\mathsf{P}}$-hard. To prove this we use the clausal program $P_\phi$ that simulates $\phi$ from Definition 15.

The rules in (12) ensure that as many candidate answer sets are generated as there are interpretations of $X_1$. The rules from (13) verify whether, for the chosen interpretation of $X_1$, it holds that $p(X_1, X_2)$ is satisfied for all interpretations of $X_2$. To see this, we first draw the attention of the reader to the fact that these rules are exactly the construct used in Proposition 13 to simulate entailment. Hence we are only able to derive '*sat*' if the set of propositional clauses $\{\neg\theta_1, ..., \neg\theta_n\}$ is unsatisfiable. Notice furthermore that the set $\{\neg\theta_1, ..., \neg\theta_n\}$ is unsatisfiable iff formula $p(X_1, X_2)$ is false. Finally, the rule (14) eliminates every answer set in which '*sat*' is not true. Thus the program $P_\phi$ only has answer sets from which '*sat*' can be entailed or it does not have any answer sets at all. Hence the problem of deciding whether a clause '*sat*' is entailed by an answer set $M$ of $P_\phi$ corresponds to determining whether or not a QBF of the form $\phi = \exists X_1 \forall X_2 \cdot p(X_1, X_2)$ is satisfiable. □

*Proposition 15* (*weak disjunction; brave reasoning*)
Let $P$ be a clausal program. The problem of deciding whether a clause '$e$' is entailed by a consistent answer set $M$ of $P$ is in $\Sigma_2^{\mathsf{P}}$.

*Proof*
To show that this problem is indeed in $\Sigma_2^{\mathsf{P}}$, we construct an algorithm to decide whether a clause '$e$' is entailed by an answer set $M$ of $P$:

```
guess a subset E of {head(r) | r ∈ P}
verify that this interpretation is an answer set as follows:
   calculate the reduct P^E of the clausal program P
   calculate the fixpoint (P^E)*_w
   verify that E is entailed by (P^E)*_w
```

The first step of the algorithm requires a choice and makes our algorithm non-deterministic. Next, we verify whether this guess is indeed an answer set which involves taking the reduct (which can be done in polynomial time), computing the fixpoint (which depends on entailment, an NP-complete problem) and finally determining whether our guess is entailed by this fixpoint (which we found in Corollary 1 to be a problem that is $\mathsf{BH}_2$-complete). The penultimate and last step thus require the use of an oracle that can solve NP problems in constant time. Hence we find that the problem of deciding whether a clause '$e$' is entailed by an answer set $M$ of $P$ is indeed in $\Sigma_2^{\mathsf{P}}$. □

*Corollary 3* (*weak disjunction; answer set existence*)
Determining whether a clausal program $P$ has a consistent answer set is an $\Sigma_2^{\mathsf{P}}$-complete problem.

*Proof*
Notice that in the proof of Proposition 16 the program $P_\phi$ only has answer sets from which '*sat*' can be entailed or that it does not have any answer sets at all. Hence the problem of determining the satisfiability of a QBF of the form $\phi = \exists X_1 \forall X_2 \cdot p(X_1, X_2)$ with $p(X_1, X_2)$ in DNF can be reduced to the problem of deciding answer set existence for a clausal program $P$. □

## References

Banerjee, M. and Dubois, D. 2009. A simple modal logic for reasoning about revealed beliefs. In *Proceedings of the 10th European Conference on Symbolic and Quantitative Approaches to Reasoning with Uncertainty (ECSQARU'09)*. 805–816.

Huth, M. and Ryan, M. 2004. *Logic in Computer Science: Modelling and Reasoning about Systems.* Cambridge University Press.

Nguyen, L. A. 2005. On the complexity of fragments of modal logics. In *Proceedings of the 5th International Conference on Advances in Modal logic (AiML'05)*. 249–268.
